# Supplementary material for: The connected Grundy coloring problem: Formulations and a local-search enhanced biased random-key genetic algorithm
Source: arXiv:2411.14533 source file (2024-11-21)
Supplement: Supplementary file 1 [file 92_appendice_brkga_novo.tex]

\section{old results - BRKGA}
