# Supplementary material for: The connected Grundy coloring problem: Formulations and a local-search enhanced biased random-key genetic algorithm
Source: arXiv:2411.14533 source file (2024-11-21)
Supplement: Supplementary file 2 [file 97_test_appendice_image.tex]

\section{Somente para testar e deixar salvo o formato geral}
\MateusF{Não estão padronizadas ainda não}

\begin{figure}
    \centering
    \includegraphics[width=0.5\linewidth]{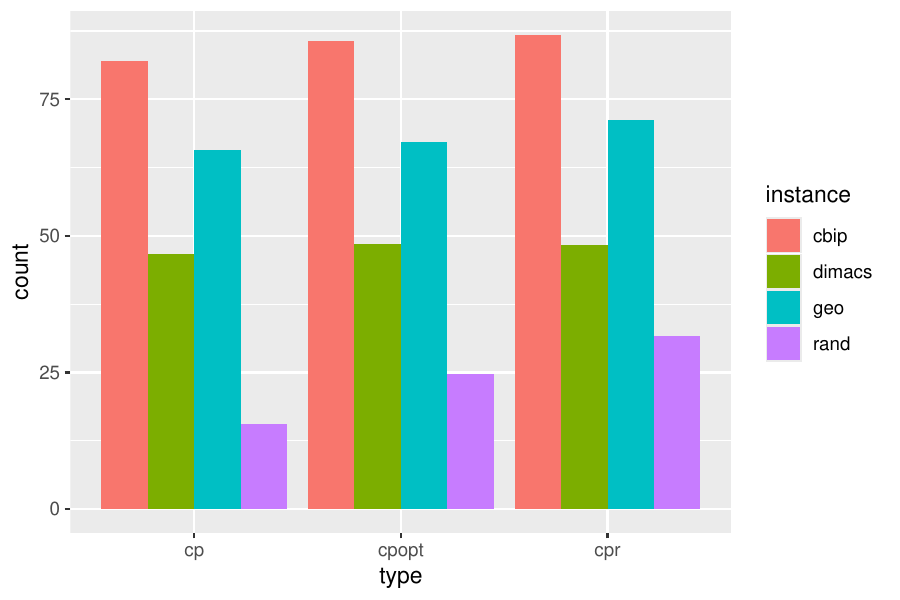}
    \caption{Caption}
    %\label{fig:enter-label}
\end{figure}

\begin{figure}
    \centering
    \includegraphics[width=0.5\linewidth]{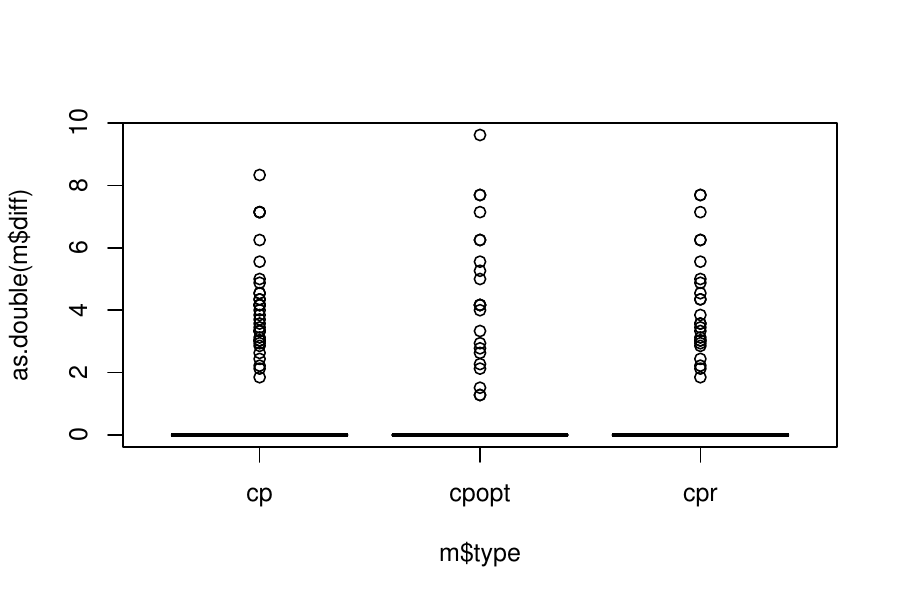}
    \caption{Caption}
    %\label{fig:enter-label}
\end{figure}

\begin{figure}
    \centering
    \includegraphics[width=0.5\linewidth]{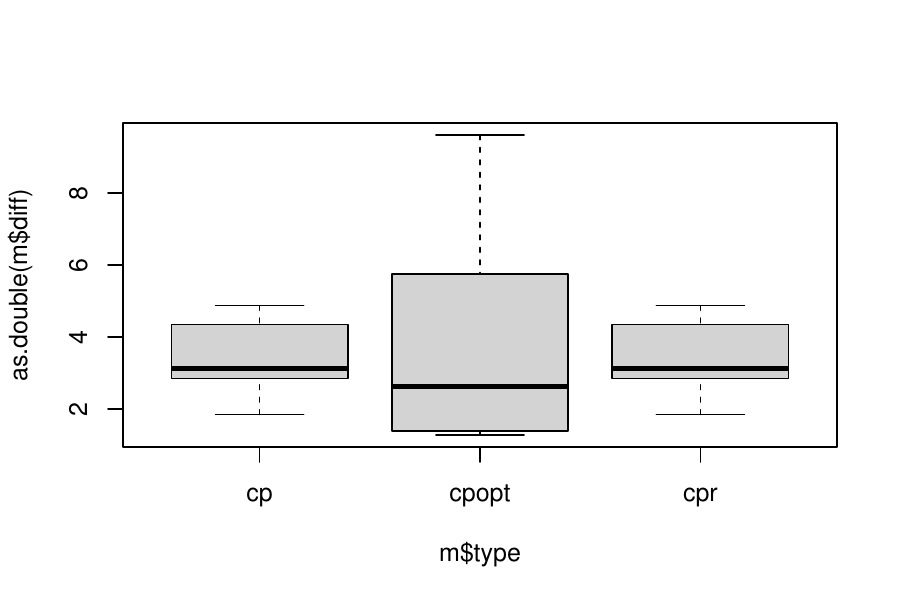}
    \caption{Caption}
    %\label{fig:enter-label}
\end{figure}

\begin{figure}
    \centering
    \includegraphics[width=0.5\linewidth]{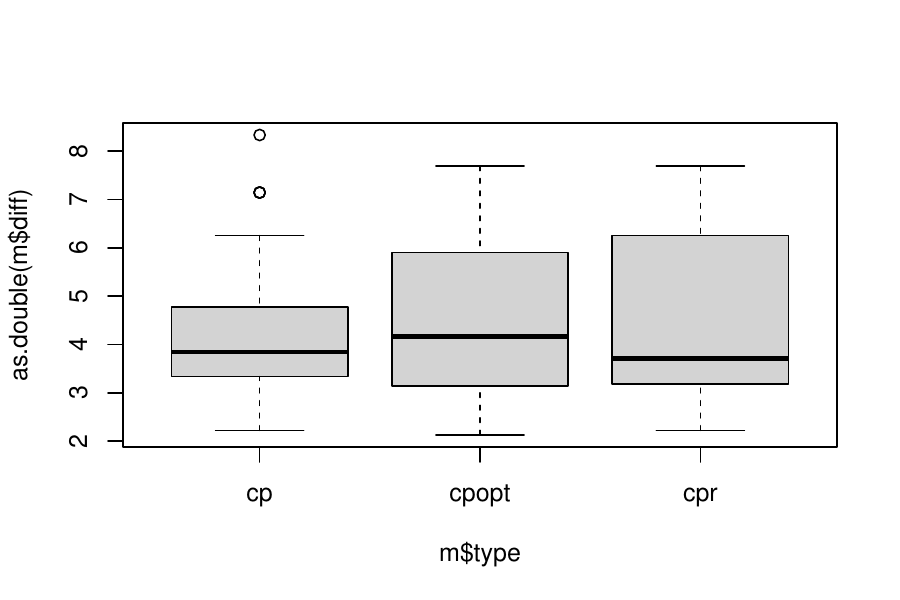}
    \caption{Caption}
    %\label{fig:enter-label}
\end{figure}
